# Supplementary material for: 50 Ways to Bake a Cookie: Mapping the Landscape of Procedural Texts
Source: arXiv:2210.17235 source file (2022-10-31)
Supplement: Supplementary file 1 [file 6_appendix.tex]

\newpage
\section{Technical Appendix} \label{appendix}

\subsection{Parser technical implementation details}
\label{app:parser}

\subsection{Clustering: Candidate pairs of instructions filtering}
\label{app:cluster}

As mentioned in Section~\ref{similarity_measure},
% \dnote{ref!!!}
we decided to take advantage of the structure extracted by our parser and create filtered list of \textit{candidate} pairs of instructions.  We require that two instructions could be considered for the same cluster only if the verbs are similar and they share enough ingredients (where ingredients that are common for the dish, such as apples count more than the rare ones). In the following, we explain the filtering steps.

\xhdr{Verb similarity}
% To produce instruction embeddings, we simply averaged all the word vectors in the instruction. 
As word embedding models achieve poor performance on verbs \cite{schwartz2016symmetric},
we manually clustered the most frequent $100$ verbs in the data
and chose a representative verb per cluster. Then, we replaced verbs in the instructions with their representative.
%before producing the instruction's embedding by simply averaging all the word vectors in the instruction. 
%The manual clustering step significantly improved the overall clustering results.

\xhdr{Similarity of two ingredient objects}
To determine whether two ingredient objects are similar, we take into account their full ingredient names ($i_f^1, i_f^2$ correspondingly) and abbreviations ($i_a^1, i_a^2$), and check if:
% Formally, we consider two ingredient objects to be similar if: 
\begin{displaymath}
max{\left(J\left(i_f^1,i_f^2\right),\ J\left(i_f^1,i_a^2\right),\ J\left(i_a^1,i_f^2\right),J\left(i_a^1,i_a^2\right)\right)}\geq t_1
\end{displaymath}
where $t_1\in[0,1]$ is a threshold and $J$ is the Jaccard index\footnote{$J(X,Y)=\frac{\left|X\cap Y\right|}{\left|X\cup Y\right|}$. In our case, $X,Y$ are the words in the ingredient name/abbreviation.}. For instance, for the name-abbreviation pairs: 
% if the name and abbreviation of two ingredients are:
(grand smith apple, apple) and (red apple, apple) 
% respectively; they are undoubtedly similar as 
% are counted similar as 
the similarity is 1. % (which is greater than every $t_1\in[0,1]$). 

\xhdr{Similarity of two ingredient sets}
Let $I_1,I_2$ be two sets of ingredient objects; to measure their similarity, we use the weighted Jaccard similarity coefficient\footnote{$J_W(x,y)=\frac{\sum_j min(x_j,y_j)}{\sum_j max(x_j, y_j)}$ for two real vectors $x,y$.}  (also known as Ruzicka similarity), taking into account also the frequency of the items in $\mathcal{S}$. This coefficient can be restated as:
\begin{displaymath}
J_W\left(I_1,I_2\right):=\frac{\sum_{x\in I_1\cap I_2}\left(n_{x}\right)}{\sum_{y\in I_1\cup I_2}\left(n_{y}\right)}
\end{displaymath}
where $n_{x}$ is the number of recipes in which ingredient $x$ appears.

We consider $I_1,I_2$ to be similar if $J_W(I_1, I_2)>t_2$ for a threshold $t_2\in[0,1]$.
Note that to calculate $J_W(I_1, I_2)$, the threshold $t_1$ must be set in advance. 
That is because computing ingredients' intersection or union expects knowing for every pair of ingredients $i_1\in I_1, i_2\in I_2$ whether they are similar or not.
We used Grid-Search on a dataset of 180 manually tagged ingredient list pairs to set values for these two hyperparameters (with bounds: 0-1), setting $t_1=0.35, t_2=0.325$.
%
% For instance, 
% let us go back to the three instructions 

% Recall the example from the beginning of this section. 
% The instructions' ingredients are:
% $I_1=$\{apples, sugar, cinnamon\}, $I_2=$\{apples, sugar, cinnamon, allspice, clove, nutmeg\},  $I_3=$\{flour, baking powder, cinnamon, clove, allspice, nutmeg\}.
% Let the instructions' ingredient sets be $I_1, I_2, I_3$ respectively. 
% Assume apples, sugar and flour are more common in $\mathcal{S}$. As $I_1$ and $I_2$ share more frequent ingredients, we get $J_W(I_1,I_2) \gg J_W(I_2,I_3)$ (and that is even though $I_2$ and $I_3$ share more ingredients in total).
% Assuming apples appears 175 times in the multiple recipe set, flour 165 times, cinnamon 161, sugar 138, baking powder 83, nutmeg 53, clove 21, and allspice 17; then, $J_w(I_1,I_2)=\frac{175+138+161}{175+138+161+53+17+21}\approx0.84$ and $J_W(I_2,I_3)\approx 0.31$. i.e, because $I_1$ and $I_2$ share more frequent ingredients, their similarity score is higher (even though $I_2$ and $I_3$ share more ingredients in total). 

\subsection{Pruning and noise reduction}
\label{app:noise}

The graph is often too large to visualize effectively. To compress it, we first prune small clusters and weak edges (nodes / edges with weight $\le 2$) that are not informative to our summary.
We also remove edges such that $w\left(a,b\right)<w\left(b,a\right)$ (i.e., we keep only the heavier edge between every two nodes in the graph), together with nodes and edges that do not belong to a path from START to END.

%Similarly, we prune edges with weak support, and edges $e=\left(a,b\right)\in E$ such that $w\left(a,b\right)<w\left(b,a\right)$).
% are also deleted (i.e., we keep only the heavier edge between every two nodes in the graph). 
 
%
% After filtering non-informative entities, we turn to 
Finally, we choose 20 dominant paths from \nstart\ to \nend.
% to display to the user. 
Picking out the heaviest simple paths in a graph is an NP-hard problem.
We drew inspiration from a heuristic that was presented  in~\cite{filippova2010multi}, inverting the edge weights and searching for the shortest paths (in terms of the edge weights).
% Too short paths 
As the order between some instructions is not important, there is some redundancy in the edge structure that can cause for the appearance of too short paths from \nstart\ to \nend\ that do not represent a reasonable recipe. Hence, we generate $K$-shortest paths (with sufficient big $K=60$) and filter those 
% We find 60 such paths using the K-shortest paths algorithm and filter all those
shorter than predefined minimal length bound\footnote{We set this bound to be the minimal recipes' number of instructions after trimming 10\% of the smallest values.}. 
The remaining paths are then reranked by normalizing their weights over their lengths. This way we obtain the paths which have the lightest average edge weight. The highest 20 paths are chosen to compose the graph displayed to the user.
